# Supplementary material for: Improved Optimistic Algorithms for Logistic Bandits
Source: arXiv:2002.07530 source file (2020-06-08)
Supplement: Supplementary file 1 [file appendix_fixed_design.tex]

\section{Fixed-design setting}
\todo{ write down the result in a Lemma distinguishing the two prediction error analysis}
\todo{ write the asymptotic analysis in $c_\mu$ and $e^S$}\\
\todo{ add Bernstein/Hoeffding inequalities to appendix}\\

We consider here the case where $x_1,\hdots, x_{T}$ are deterministic - also known as the \emph{fixed-design} setting. The purpose of this section is to expose the scaling that is attainable in this simplified setting to gain intuition on what we should expect in the \emph{adaptive} design case. We are interested in the prediction error:
\begin{align}
    \Delta_t \defeq \mu(x_t^T\theta_*) - \mu(x_t^T\hat{\theta})
\end{align}
and its cumulative behavior. As shown before through the mean value theorem and the optimality conditions for $\hat{\theta}_t$ we have that:
\begin{align}
    \Delta_t &= \alpha_t(x_t)x_t^T(\hat{\theta}_t-\theta_*)\\
    &= \alpha_t(x_t) x_t^T\tilde{\mbold{G}}_{t}^{-1}S_t\\
    &\leq \frac{1}{4} \sum_{s=1}^{t-1}\varepsilon_sx_t^T\tilde{\mbold{G}}_{t}^{-1}x_s
\end{align}
The only random quantities in the sum above are the $\{\epsilon_s\}$, and we can therefore apply standard concentration inequalities. Because the $\{\varepsilon_s\}_{s=1}^\infty$ are Bernoulli random variables they are therefore $1/2$-subGaussian. Also, a naive application of Hoeffding inequality yields that for $\varepsilon>0$:
\begin{align}
   \mathbb{P}\left( \sum_{s=1}^{t-1}\varepsilon_sx_t^T\tilde{\mbold{G}}_{t}^{-1}x_s\geq \varepsilon\right) \leq \exp\left(\frac{-\varepsilon^2}{8\sum_{s=1}^{t-1}\left(x_t^T\tilde{\mbold{G}}_{t}^{-1}x_s\right)^2}\right)
\end{align}
Therefore for $\delta\in(0,1)$, with probability at least $1-\delta$:
\begin{align}
    \sum_{s=1}^{t-1}\varepsilon_sx^T\tilde{\mbold{G}}_{t}^{-1}x_s \leq 2\sqrt{2\log(1/\delta)}\sqrt{x_t^T\tilde{\mbold{G}}_{t}^{-1}V_t\tilde{\mbold{G}}_{t}^{-1}x_t}
\end{align}
A close path to the one followed by \cite{filippi2010parametric} consists in using $\tilde{\mbold{G}}_t \geq c_\mu \mbold{V}_t$. It turns out that this is the easiest strategy to follow in order to subsequently bound the cumulative sum of $\Delta_t$. We proceed:
\begin{align}
    \sum_{s=1}^{t-1}\varepsilon_sx^T\tilde{\mbold{G}}_{t}^{-1}x_s \leq \frac{2}{c_\mu}\sqrt{2\log(1/\delta)}\mnorm{x_t}{V_t^{-1}}
\end{align}
which then yields:
\begin{align}
    \Delta_t \leq \frac{1}{2c_\mu}\sqrt{2\log(1/\delta})\mnorm{x_t}{V_t^{-1}}
\end{align}
Thanks to a Cauchy-Schwartz inequality, and using the Elliptical Potential Lemma (TODO) we obtain:
\begin{align}
    \sum_{t=1}^T \Delta_t &= \tilde{\mcal{O}}\left(\frac{1}{c_\mu}\sqrt{T}\right)\\
    &= \tilde{\mcal{O}}\left(e^{S}\sqrt{T}\right)
\end{align}
with probability at least $1-\delta$. This result is of course to be linked with the one of \cite{filippi2010parametric} obtained in the adaptive setting. Note that by using an Hoeffding inequality, we obtain a result that is lagging behind the asymptotic analysis, by a $\sqrt{k_\mu/c_\mu}$ multiplicative term. It happens that a much better result can be obtained thanks to \emph{self-concordance} and the use of a Bernstein bound instead of an Hoeffding bound.

In what follows, we will assume for simplicity that $\hat{\theta}_t\in\Theta$. This approximation is not necessary but eases the discussion for now. We will not use it for the derivation of guarantees in the adaptive case. Let us apply Bernstein's inequality to $\sum_{s=1}^{t-1} \varepsilon_{s+1}x_t^T\tilde{\mbold{G}}_t^{-1}x_s$. Simple linear algebra gives that almost surely:
\begin{align}
    \vert \varepsilon_{s+1}x_t^T\tilde{\mbold{G}}_t^{-1}x_s\vert \leq \frac{X}{\sqrt{\lambda}}\left\lVert x_t\right\rVert_{\tilde{\mbold{G}}_t^{-1}}
\end{align}
Note also that:
\begin{align}
    \sum_{s=1}^{t-1} \text{Var}\left(\varepsilon_{s+1}x_t^T\tilde{\mbold{G}}_{t}^{-1}x_s\right)=x_t^T \tilde{\mbold{G}}_{t}^{-1}\left(\sum_{s=1}^{t-1}\sigma_s^2x_sx_s^T\right)\tilde{\mbold{G}}_{t}^{-1}x_t
\label{eq:bernsteinsumvariance}
\end{align}
We are going to give an upper-bound for the variance thanks to the self-concordance properties of the sigmoid function. Apply Lemma~\ref{lemma:self_concordance} with $z_1=x_s^T\theta_*$ and $z_2 = x_s^T(\hat{\theta_t}-\theta_*)$ to obtain:
\begin{align}
    \alpha_t(x_s) &\geq \dot{\mu}(x_s^T\theta_*)\left(1+x_s^T(\hat{\theta}_t-\theta_*)\right)^{-1}\\
    &\geq \dot{\mu}(x_s^T\theta_*)\left(1+2XS\right)^{-1}
\end{align}
Therefore since $\dot{\mu}(x_s^T\theta_*)= \mu(x_s^T\theta_*)(1-\mu(x_s^T\theta_*))=\sigma_s^2$:
\begin{align}
    \tilde{\mbold{G}}_t \geq (1+2XS)^{-1}\sum_{s=1}^{t-1} \sigma_s^2x_sx_s^T
\end{align}
and by replacing in Equation~\eqref{eq:bernsteinsumvariance} and some simple algebra we obtain that:
\begin{align}
    \sum_{s=1}^{t-1} \text{Var}\left(\varepsilon_{s+1}x_t^T\tilde{\mbold{G}}_{t}^{-1}x_s\right)\leq (1+2XS)\left\lVert x_t\right\rVert_{\tilde{\mbold{G}}_t^{-1}}^2
\end{align}
Then, an application of Bernstein's inequality gives that with probability at least $1-\delta$:
\begin{align}
   \Delta_t &\leq \frac{2X}{3\sqrt{\lambda}}\log(1/\delta)\left\lVert x_t\right\rVert_{\tilde{\mbold{G}}_t^{-1}} + \sqrt{(2+4XS)\log(1/\delta)}\left\lVert x_t\right\rVert_{\tilde{\mbold{G}}_t^{-1}} \\
   &\leq \frac{2X}{3\sqrt{\lambda c_\mu}}\log(1/\delta)\left\lVert x_t\right\rVert_{\mbold{V}_t^{-1}} + \sqrt{\frac{2+4XS}{c_\mu}\log(1/\delta)}\left\lVert x_t\right\rVert_{\mbold{V}_t^{-1}} 
\end{align}
which will in turn yield thanks to the Elliptic Potential Lemma:
\begin{align}
    \sum_{s=1}^T \Delta_t &= \tilde{\mcal{O}}\left(\sqrt{\frac{S}{c_\mu}}\sqrt{T}\right)\\
    &= \tilde{\mcal{O}}\left(\sqrt{Se^S}\sqrt{T}\right)
\end{align}
which is no longer lagging behind the asymptotic analysis (up to constant and logarithmic terms).
